# Supplementary material for: On wedge-slamming pressures
Source: arXiv:2011.10378 ancillary file (2021-12-11)
Supplement: Supplementary file 1 [file wedgesupplementaryresults.pdf]

## Supplementary material for ‘On wedge-slamming pressures’

Utkarsh Jain,<sup>1,\*</sup> Vladimir Novaković,<sup>2</sup> Hannes Bogaert,<sup>2</sup> and Devaraj van der Meer<sup>1</sup>

<sup>1</sup>*Physics of Fluids Group and Max Planck Center Twente for Complex Fluid Dynamics,  
MESA+ Institute and J. M. Burgers Centre for Fluid Dynamics,  
University of Twente, P.O. Box 217, 7500AE Enschede, The Netherlands*

<sup>2</sup>*Maritime Research Institute (MARIN), 6708PM Wageningen, The Netherlands*

(Dated: December 11, 2021)

This supplementary material document contains additional information and figures on air entrapment for very small deadrise-angle cones (in Section I). In Section II we discuss the air cushioning results from additional cones with deadrise angles comparable to those in the main article Figs. 10 and 12 for a cone with a deadrise angle of  $\beta = 10^\circ$ . We show additional results for the wetting rate of the cone post-impact in Section III).

### I. AIR ENTRAPMENT UNDER $1^\circ$ & $2^\circ$ DEADRISE ANGLE CONES AT SLAMMING VELOCITIES OF 1.0 M/S

The velocity profile in an air film being squeezed out from under an axisymmetric cone with a certain deadrise angle  $\beta$  that is about to slam onto water can be estimated from the depth-integrated continuity equation as

$$V_{r,\text{gas}} = \frac{r}{2} \frac{V}{V\tau + r \tan \beta}. \quad (1)$$

Ignoring any vertical air velocities in the gap, a rather strong radial (dynamic) pressure gradient in the gap is set up on account of (1). At  $r = 0$ , the dynamic pressure is zero, while the static (stagnation) pressure assumes its largest value - this deflects the water surface away from the approaching impactor.

Therefore, under the edge of the impactor, where the dynamic pressure takes its largest value (within the impactor's shadow) the static pressure has a minimum and may cause the water surface to rise on account of this low pressure.

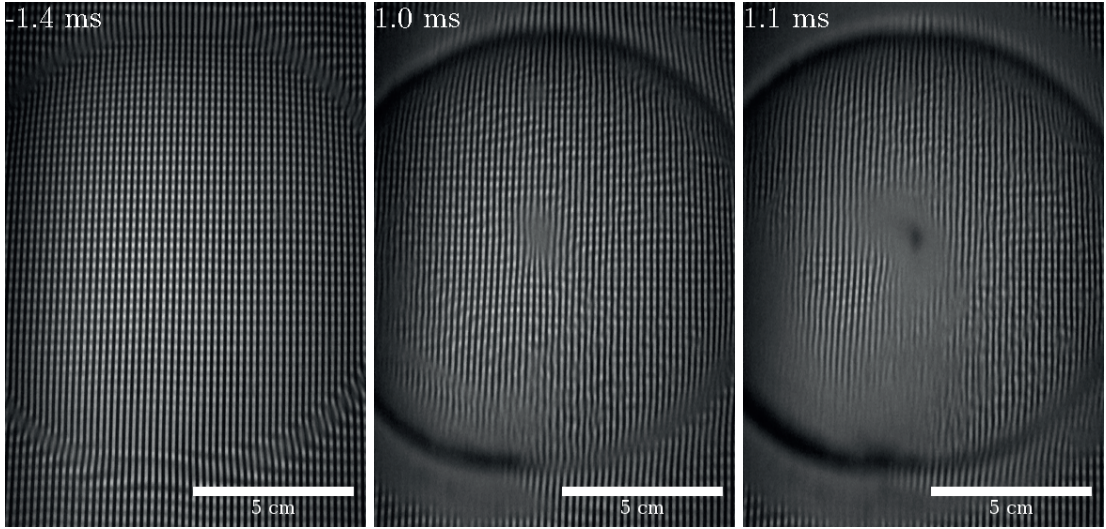

FIG. S1. Snapshots from the free surface, visualised using a total internal reflection setup prior to the impact of a cone with a diameter  $D = 14$  cm and a deadrise angle of  $\beta = 1^\circ$  at an impact velocity  $V = 1.0$  m/s. The images are time labelled such that the first contact between the cone and the water happens at  $t = 0$ . The wet parts of the cone turn black as the reflecting surface disappears from the wetted parts of the cone. In this particular case, the edge of the cone wets first (at  $t = 0.0$  ms, i.e., just before the second snapshot) followed later by the keel (just before  $t = 1.1$  ms, the third snapshot). Also see supplementary Movie 2.

---

\* [u.jain@utwente.nl](mailto:u.jain@utwente.nl)

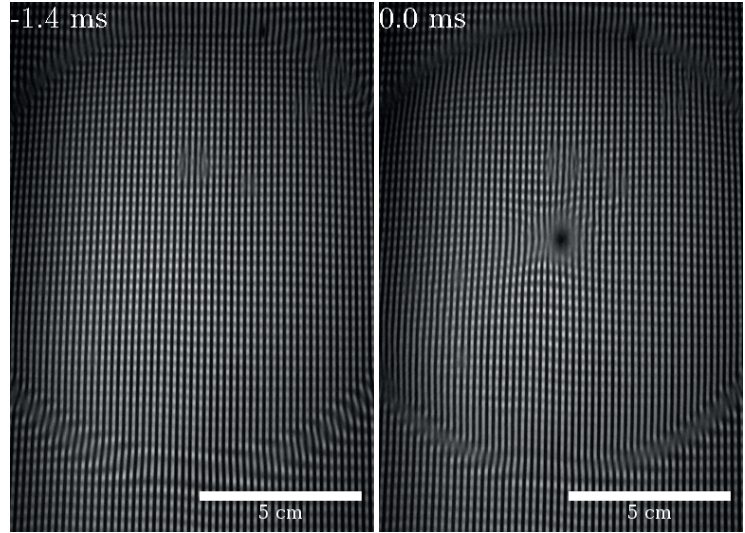

FIG. S2. Snapshots from the free surface, visualised using a total internal reflection setup prior to the impact of a cone with a diameter  $D = 14$  cm and a larger deadrise angle of  $\beta = 2^\circ$  at an impact velocity  $V = 1.0$  m/s. Again, the images are time labelled such that the first contact between the cone and the water happens at  $t = 0$ . In this second case, the keel of the cone wets first (at  $t = 0.0$  ms, just before the second snapshot) Also see supplementary Movie 3.

Depending on the shape of the water surface under the impactor at the moment of impact, the impactor may first make contact with the water at any location. Naturally, with increasing deadrise angle  $\beta$ , the radial gradient of the air pressure weakens, and the air layer's effect on the stationary free surface also weakens.

We show two such examples using cones with deadrise angles of  $1^\circ$  and  $2^\circ$ . Since the purpose now is to illustrate the trapping of air under the cone, we use larger cones than in the main article, i.e., with a diameter of 140 mm (compared to 70 mm in the main text), which enhances the visibility of the free surface deformation resulting from the air layer dynamics before impact. In figure S1 we see that, for the  $1^\circ$  cone, the edge wets first, and the keel contacts the liquid later. The wetting dynamics are completely different for even slightly higher deadrise-angle cones where the contact starts from the cone's keel: As an example we show the impact of a cone of a slightly larger deadrise angle of  $\beta = 2^\circ$  in figure S2, where the first contact with the liquid takes place at the cone's keel.

Clearly, in the case where air is entrapped below the entire cone, Wagner theories should be used with much more care. In the case of figure S2 however, where the first impact happens at the keel, the post impact dynamics of the liquid domain is very close to how they are modelled in Wagner theories.

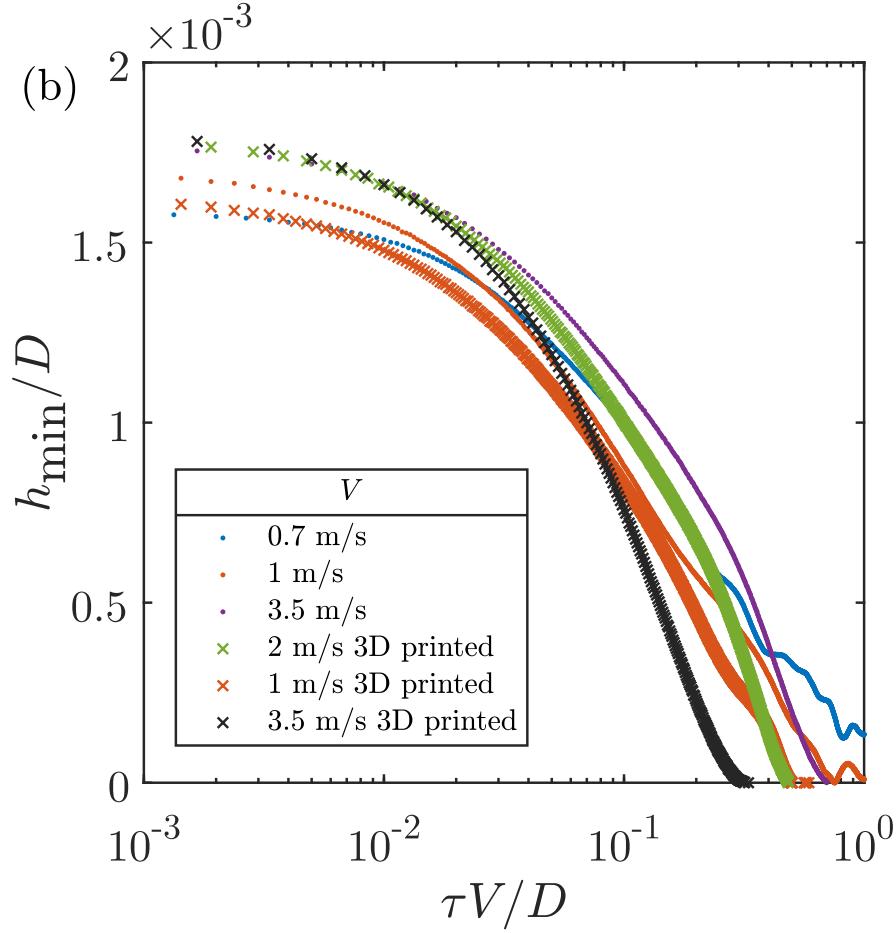

FIG. S3. Comparing the non-dimensionalised depth  $h_{\min}/D$  of the water surface deformation at  $r = 0$  below two approaching  $10^\circ$  deadrise-angle cones of different material, plotted versus the nondimensionalised time remaining until impact,  $\tau V/D = (t_{\text{impact}} - t)V/D$ , for three different impact velocities  $V$ . The results represented by the small dots were measured with the PET polyester  $10^\circ$  cones that were used for the measurements presented in the main article, and those denoted by the crosses are obtained with 3D printed cones.

## II. AIR CUSHIONING UNDER 70 MM WIDE CONES WITH $\beta = 5^\circ$ , $20^\circ$ , AND $30^\circ$ .

In the main article we presented measurements of the deformation of the water-air interface of a cone with a deadrise angle of  $\beta = 10^\circ$ . Here we extend those measurements by comparing to a cone of a different material and the same deadrise angle  $\beta = 10^\circ$ , and also by presenting equivalent measurements of cones with different deadrise angles of  $5^\circ$ ,  $20^\circ$ , and  $30^\circ$ .

First we compare the water surface deformation measured at different impact velocities  $V$  with two cones made of different materials with different surface finishes in figure S3. The first (small dots) is the same PET polyester cone that was used for the measurements presented in the main article, and with which also the pressures were measured, and the second a 3D printed cone (crosses), which is made of the same material (Formlabs Clear V4) as the cones of other deadrise angles ( $\beta = 5^\circ$ ,  $20^\circ$ , and  $30^\circ$ ) with which the air-cushioning measurements discussed in this supplementary material and the force measurements discussed in appendix A of the main article were performed. There is no observable difference between the measurements performed with the two cones and we can conclude that air-cushioning measurements performed with PET cones and 3D printed cones can be compared to each other without reservations.

Secondly, we present results of measurements of the water surface deformation for 3D printed cones with deadrise angles of  $\beta = 5^\circ$ ,  $20^\circ$ , and  $30^\circ$  cones. As in the main paper, we show the final cavity depth  $h_{\min}$  before impact using the remaining time until impact,  $\tau = t_{\text{impact}} - t$  (i.e., with reversed time direction) in the panels (a) of figures S3–S6 and in the insets we show that the data collapses when non-dimensionalised with inertial scales. In the other panels of figures S3–S6 we show the same data compared to boundary integral simulations, now using forward time  $t$ . After

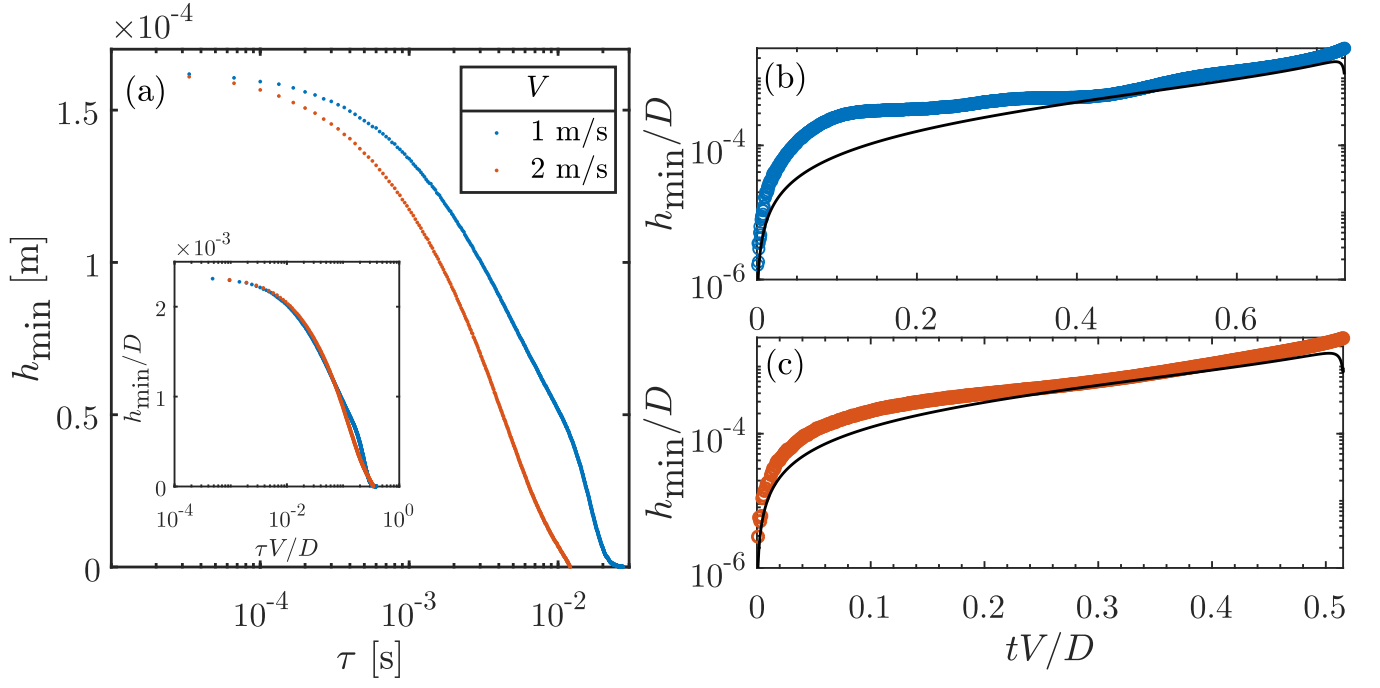

FIG. S4. (a) Experimentally measured central depth  $h_{\min}$  of the deformed water surface at  $r = 0$  below an approaching cone with a deadrise angle of  $\beta = 5^\circ$  is plotted versus the time remaining until impact,  $\tau = t_{\text{impact}} - t$ , for two different impact velocities  $V$ . The inset shows the collapse of the same data when nondimensionalised using inertial scales. In panels (b–c) we compare the results from panel (a) (same colour coding) with  $h_{\min}$  determined from two-fluid boundary integral simulations, now using forward time  $t$ .

a short start-up period, the potential flow simulations reproduce the experimentally measured free surface deflection well until the very late stages, when the two-fluid interface in the BI diverges due to numerical issues.

For each deadrise angle  $\beta$ , the final depths  $h_{\min}$  obtained just before impact are collected from the above results, nondimensionalised and plotted as figure 13 in the main article where the variation of cavity depth with  $\beta$  is discussed.

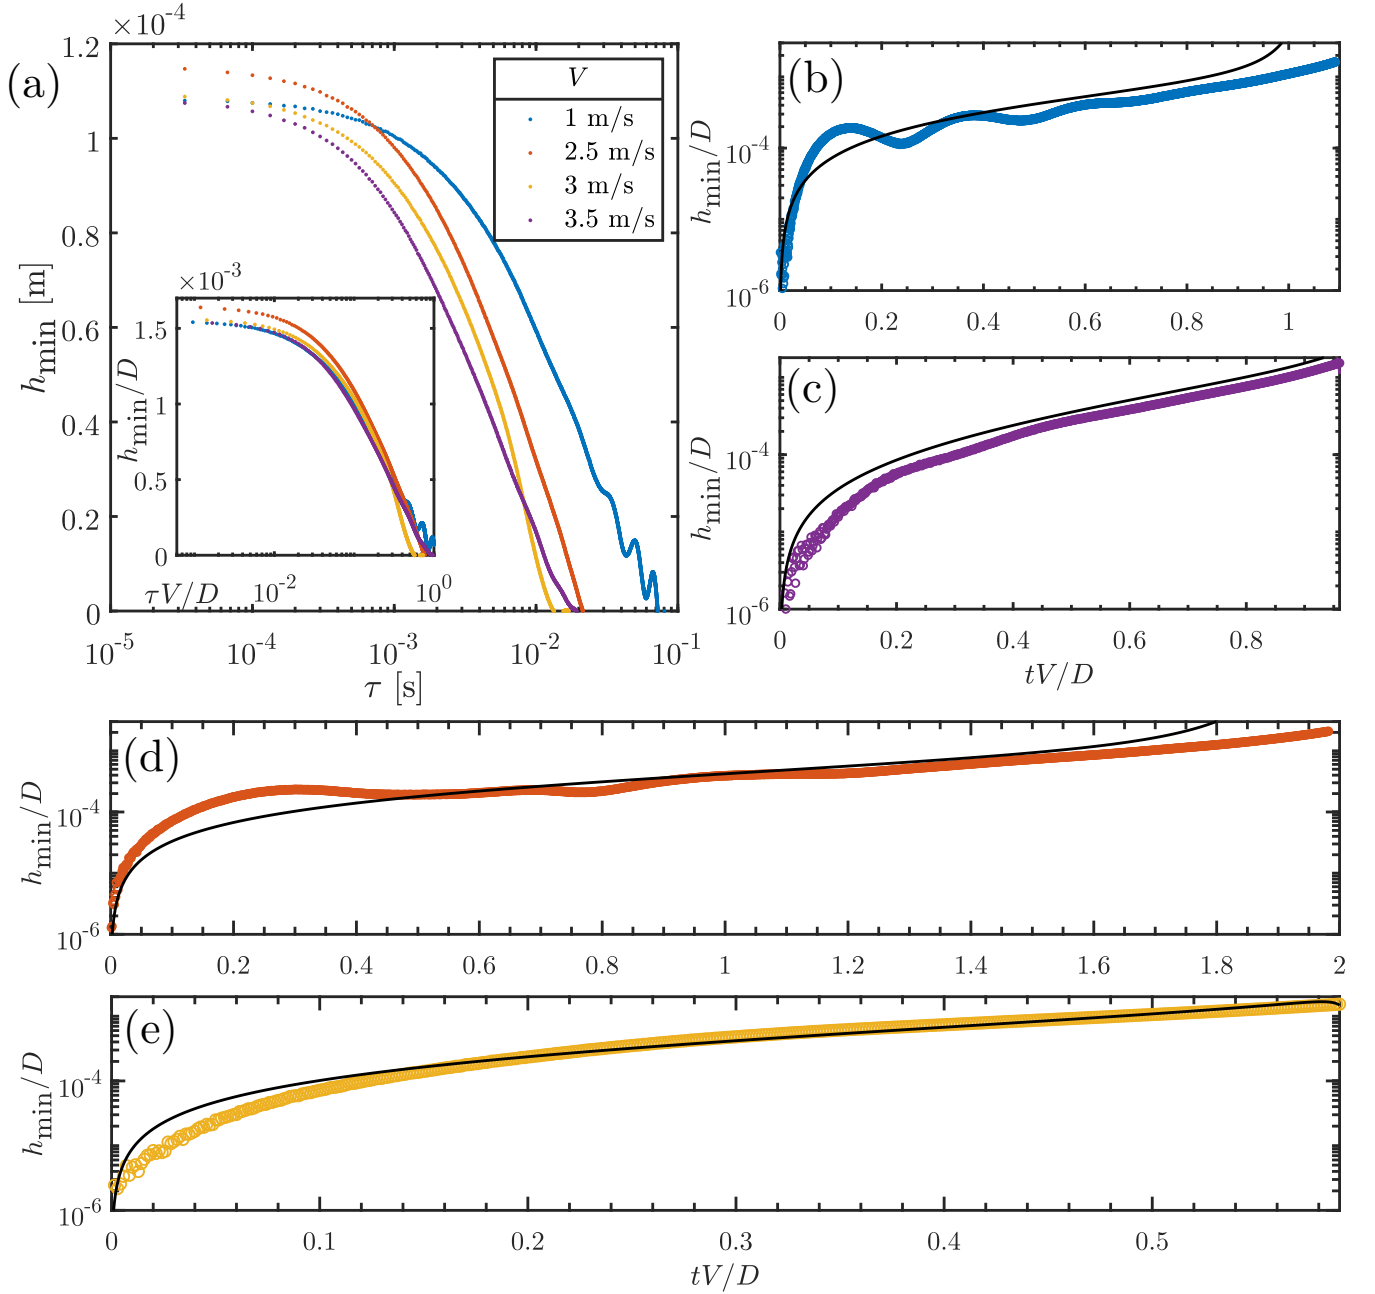

FIG. S5. (a) Experimentally measured central depth  $h_{\min}$  of the deformed water surface at  $r = 0$  below an approaching cone with a deadrise angle of  $\beta = 20^\circ$  is plotted versus the time remaining until impact,  $\tau = t_{\text{impact}} - t$ , for four different impact velocities  $V$ . The inset shows the collapse of the same data when nondimensionalised using inertial scales. In panels (b–e) we compare the results from panel (a) (same colour coding) with  $h_{\min}$  determined from two-fluid boundary integral simulations, now using forward time  $t$ .

### III. WETTING RATE OF CONES WITH $\beta = 5, 20, 30^\circ$

Using the total-internal-reflection setup after impact, we followed the same procedure as discussed in the main article for a cone with a deadrise angle of  $10^\circ$  to measure the widths of the wetted section of all the deadrise angle cones, and plot the results in figure S7 alongside the Wagner [1–3] condition

$$c(t) = \frac{4Vt}{\pi \tan \beta}, \quad (2)$$

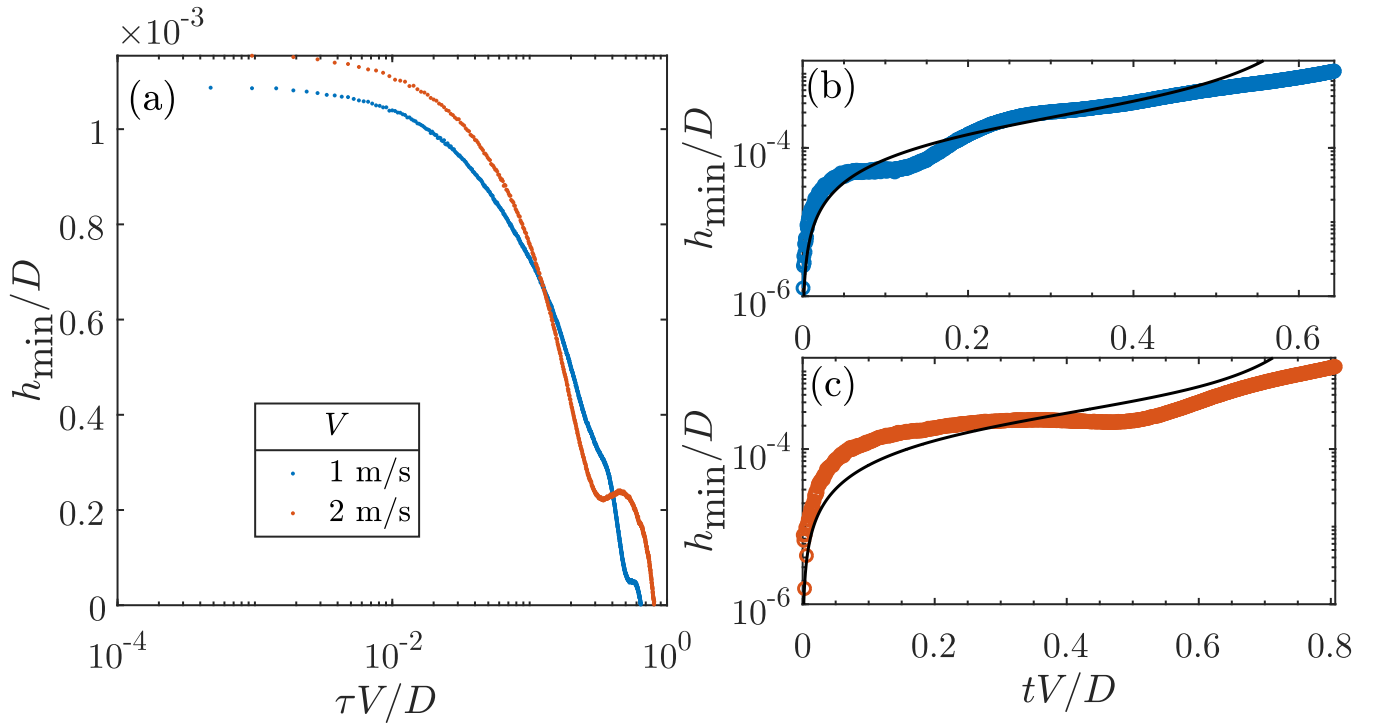

FIG. S6. (a) Experimentally measured central depth  $h_{\min}$  of the deformed water surface at  $r = 0$  below an approaching cone with a deadrise angle of  $\beta = 30^\circ$  is plotted versus the time remaining until impact,  $\tau = t_{\text{impact}} - t$ , for two different impact velocities  $V$ . The inset shows the collapse of the same data when nondimensionalised using inertial scales. In panels (b–c) we compare the results from panel (a) (same colour coding) with  $h_{\min}$  determined from two-fluid boundary integral simulations, now using forward time  $t$ .

which predicts the wetting rate of a water-entering cone. We find very good agreement between the measurements and the theoretical prediction for all measured deadrise angles ( $\beta = 5^\circ, 10^\circ, 20^\circ$ , and  $30^\circ$ ).

- 
- [1] Herbert Wagner. Über stoß-und gleitvorgänge an der oberfläche von flüssigkeiten. *Z. Angew. Math. Mech.*, 12(4):193–215, 1932.
  - [2] C. Schmieden. Der aufschlag von rotationskörpern auf eine wasseroberfläche. richard v. mises zum 70. geburtstag gewidmet. *ZAMM - Journal of Applied Mathematics and Mechanics / Zeitschrift für Angewandte Mathematik und Mechanik*, 33(4):147–151, 1953.
  - [3] O. Faltinsen and R. Zhao. Water entry of ship sections and axisymmetric bodies. In *AGARD REPORT 827 High Speed Body Motion in Water*, 1998.

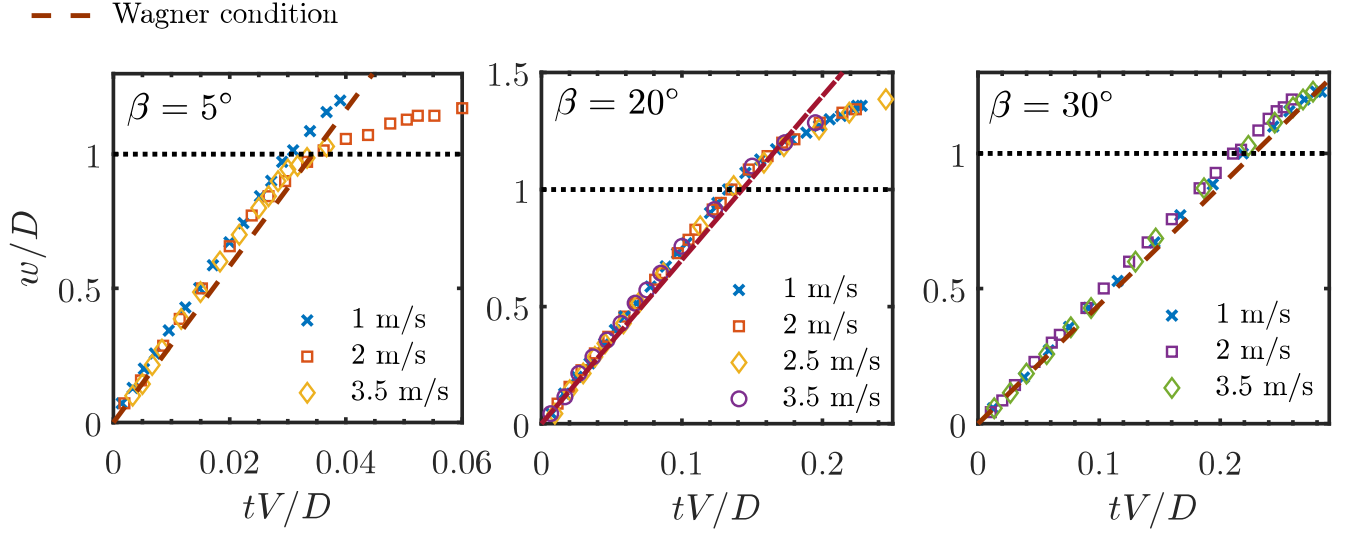

FIG. S7. Dimensionless wetted width  $w/D$  as a function of dimensionless time  $tV/D$  for cones with (a)  $5^\circ$ , (b)  $20^\circ$  and (c)  $30^\circ$  deadrise angles, together with the Wagner condition Eq. (2) (magenta dashed lines). Each panel contains experiments at different impact velocities  $V$ .
